# Supplementary material for: Les Houches 2023: Physics at TeV Colliders: Standard Model Working Group Report
Source: arXiv:2406.00708 source file (2024-06-02)
Supplement: Supplementary file 1 [file sm_pheno.packages.tex]

% add here the packages you used locally, 1 package per line

%\usepackage{xcolor}
%\usepackage{booktabs}
%\usepackage{arydshln}
